# Supplementary material for: Grey-box models for wave loading prediction
Source: arXiv:2105.13813 source file (2021-06-30)
Supplement: Supplementary file 1 [file Appendix.tex]

\subsection{Morison's Equation}
Morison's equation has provided a widely used tool for the modelling of wave loading on slender members since it's introduction in 1950 \cite{Morison1950}.
Morison's equation for cylinder:
\begin{equation}
F(t) = \underbrace{\frac{1}{2}\rho DC_d}_{\begin{matrix}{C_d'}\end{matrix}}u|u| + \underbrace{\frac{1}{4}\pi\rho D^2C_m}_{\begin{matrix}{C_m'}\end{matrix}}\dot{u}
\end{equation}
Although quick to compute, Morison's Equation relies on a number of simplifying assumptions:
\begin{itemize}
  \item The waves are not affected by the presence of the submerged members. For a cylindrical structure, the wavelength should far exceed the diameter \cite{MorisonAsumpSlender}.
  \item Another entry in the list
\end{itemize} 
Simplified form:
\begin{equation}
F(t) = C_d'u|u| + C_m'\dot{u}
\end{equation}

\subsection{Gaussian Processes}
Mean and covariance functions:
\begin{equation}
m(x) = \mathop{\mathbb{E}}[f(x)]
\end{equation}
\begin{equation}
k(x,x') = \mathop{\mathbb{E}}[(f(x)-m(x))(f(x')-m(x'))]
\end{equation}
Gaussian Process:
\begin{equation}
f(x) = \mathcal{GP}(m(x),k(x,x'))
\end{equation}
Gaussian process with noisy observations:
\begin{equation}
\begin{bmatrix}
y\\ f_*
\end{bmatrix} \sim \mathcal{N}
\begin{pmatrix}
0, & \begin{bmatrix}
K(X,X) + \sigma^2_n I& K(X,X_*)\\ 
K(X_*,X) & K(X_*,X_*)
\end{bmatrix}
\end{pmatrix}
\end{equation}
\subsection{Autoregressive Models}
AR - only lagged output values - linear
\begin{equation}
y_t = \alpha_1y_{t-1} + \alpha_2y_{t-2} + ... + \alpha_{l_y}y_{t-l_y} + \varepsilon_t = \sum_{i=1}^{l_u}\alpha _iy_{t-i} + \varepsilon_t
\end{equation}
ARX - both lagged inputs and outputs - linear
\begin{equation}
y_t = \sum_{i=0}^{l_u}\alpha _iu_{t-i} + \sum_{i=1}^{l_y}\beta _iy_{t-i} + \varepsilon_t
\end{equation}
NARX - both lagged inputs and outputs - used inside non-linear function
\begin{equation}
y_t = f(u_{t},u_{t-1},u_{t-2},...,u_{t-l_u},y_{t-1},y_{t-2},...,y_{t-l_y}) + \varepsilon_t
\end{equation}
\subsection{GP-NARX}
NARX model - uses a GP as the non-linear function
\begin{equation}
y_t = \mathcal{GP}(u_{t},u_{t-1},u_{t-2},...,u_{t-l_u},y_{t-1},y_{t-2},...,y_{t-l_y}) + \varepsilon_t
\end{equation}
Uses of NARX in literature ... \\
Types of prediction - MPO vs OSA - maybe draw the loop diagram

\subsection{Dataset Spectral Analysis}
Selected univariate loading section - explain why\\
Compare spectra - explain why\\
Pwelch settings - 16 windows, hamming window, no overlap - justify
\begin{figure}[ht]
  \centering
      \includegraphics[width=1\textwidth]{Spectra_Pwelch_Dataset_Comparison.png}
  \caption{Spectra Pwelch Dataset Comparison.}
  \label{fig:Pwelch_Datasets}
\end{figure}

Pearson's correlation coefficient:
\begin{equation}
r_{A,B} = \frac{n\sum_{i=1}^{n}A_iB_i - \sum_{i=1}^{n}A_i\sum_{i=1}^{n}B_i}{\sqrt{n\sum_{i=1}^{n}A_i^2-(\sum_{i=1}^{n}A_i)^2}\sqrt{n\sum_{i=1}^{n}B_i^2-(\sum_{i=1}^{n}B_i)^2}}
\end{equation}
\begin{table}[ht]
\sisetup{round-mode=places,round-precision=3}
  \begin{center}
    \caption{Pearson's correlation coefficient for velocity, acceleration and force spectra between training, validation and test datasets.}
    \label{tab:pearson}
    \begin{tabular}{lSSS} % <-- Changed to S here.
    \toprule
      \textbf{Comparison} & \textbf{Velocity} & \textbf{Acceleration} & \textbf{Force}\\
      \midrule
    Training-Validation  &  0.91267    &   0.91477   &    0.77125\\
    Training-Test    &      0.93157    &   0.87585   &    0.88436\\
    Validation-Test   &     0.96085    &   0.97311   &    0.93387\\
      \bottomrule
    \end{tabular}
  \end{center}
\end{table}

Cosine similarity
\begin{equation}
cos(\theta )=\frac{A\cdot B}{\left \| A \right \|\left \| B \right \|}=\frac{\sum_{i=1}^{n}A_iB_i}{\sqrt{\sum_{i=1}^{n}A_i^2}\sqrt{\sum_{i=1}^{n}B_i^2}}
\end{equation}

\begin{table}[ht]
\sisetup{round-mode=places,round-precision=3}
  \begin{center}
    \caption{Cosine similarity for velocity, acceleration and force spectra between training, validation and test datasets.}
    \label{tab:cos_sim}
    \begin{tabular}{lSSS} % <-- Changed to S here.
    \toprule
      \textbf{Comparison} & \textbf{Velocity} & \textbf{Acceleration} & \textbf{Force}\\
      \midrule
    Training-Validation &   0.91753   &    0.92045   &    0.78781\\
    Training-Test     &     0.93586   &    0.88438   &    0.89296\\
    Validation-Test    &    0.96278   &    0.97522   &    0.93885\\
      \bottomrule
    \end{tabular}
  \end{center}
\end{table}

\newpage
\appendix
\counterwithin{figure}{section}
\section{Appendix}
\subsection{Model posterior plots}
\begin{figure}[ht]
  \centering
  \includegraphics[width=1\textwidth]{White_Box_Lin_Reg.png}
  \caption{White-box linear regression on test dataset.}
  \label{fig:White_Box_Lin_Reg}
  
  \includegraphics[width=1\textwidth]{White_Box_ARX_OSA.png}
  \caption{White-box ARX OSA prediction on test dataset.}
  \label{fig:White_Box_ARX_OSA}
\end{figure}

\newpage
\begin{figure}[ht]
  \centering
  \includegraphics[width=1\textwidth]{White_Box_ARX_MPO.png}
  \caption{White-box ARX MPO prediction on test dataset.}
  \label{fig:White_Box_ARX_MPO}
  
  \includegraphics[width=1\textwidth]{Black_Box_GP_Static_Train_1000.png}
  \caption{Black-box static GP prediction on test dataset.}
  \label{fig:Black_Box_GP_Static}
\end{figure}

\newpage
\begin{figure}[ht]
  \centering
  \includegraphics[width=1\textwidth]{Black_NARX_mpo_1000_MC_1000_OSA_Conf.png}
  \caption{Black-box GP-NARX OSA prediction on test dataset.}
  \label{fig:Black_Box_GP-NARX_OSA}

  \includegraphics[width=1\textwidth]{Black_NARX_mpo_1000_MC_1000_Mean_Conf.png}
  \caption{Black-box GP-NARX MPO prediction on test dataset.}
  \label{fig:Black_Box_GP-NARX_MPO}
\end{figure}

\newpage
\begin{figure}[ht]
  \centering
  \includegraphics[width=1\textwidth]{Black_NARX_mpo_1000_MC_1000_MC_Conf.png}
  \caption{Black-box GP-NARX MC MPO prediction on test dataset.}
  \label{fig:Black_Box_GP-NARX_MC}

  \includegraphics[width=1\textwidth]{Grey_bias_GP_Static_Train_1000.png}
  \caption{Grey-box bias correction static GP prediction on test dataset.}
  \label{fig:Grey_Box_GP_bias}
\end{figure}

\newpage
\begin{figure}[ht]
  \centering
  \includegraphics[width=1\textwidth]{Grey_bias_NARX_mpo_1000_MC_1000_OSA_Conf.png}
  \caption{Grey-box bias correction GP-NARX OSA prediction on test dataset.}
  \label{fig:Grey_Box_GP-NARX_OSA_bias}

  \includegraphics[width=1\textwidth]{Grey_bias_NARX_mpo_1000_MC_1000_Mean_Conf.png}
  \caption{Grey-box bias correction GP-NARX MPO prediction on test dataset.}
  \label{fig:Grey_Box_GP-NARX_MPO_bias}
\end{figure}

\newpage
\begin{figure}[ht]
  \centering
  \includegraphics[width=1\textwidth]{Grey_bias_NARX_mpo_1000_MC_1000_MC_Conf.png}
  \caption{Grey-box bias correction GP-NARX MC MPO prediction on test dataset.}
  \label{fig:Grey_Box_GP-NARX_MC_bias}

  \includegraphics[width=1\textwidth]{Grey_input_GP_Static_Train_1000.png}
  \caption{Grey-box input augmentation static GP prediction on test dataset.}
  \label{fig:Grey_Box_GP_input}
\end{figure}

\newpage
\begin{figure}[ht]
  \centering
  \includegraphics[width=1\textwidth]{Grey_input_NARX_mpo_1000_MC_1000_OSA_Conf.png}
  \caption{Grey-box input augmentation GP-NARX OSA prediction on test dataset.}
  \label{fig:Grey_Box_GP-NARX_OSA_input}

  \includegraphics[width=1\textwidth]{Grey_input_NARX_mpo_1000_MC_1000_Mean_Conf.png}
  \caption{Grey-box input augmentation GP-NARX MPO prediction on test dataset.}
  \label{fig:Grey_Box_GP-NARX_MPO_input}
\end{figure}

\newpage
\begin{figure}[ht]
  \centering
      \includegraphics[width=1\textwidth]{Grey_input_NARX_mpo_1000_MC_1000_MC_Conf.png}
  \caption{Grey-box input augmentation GP-NARX MC MPO prediction on test dataset.}
  \label{fig:Grey_Box_GP-NARX_MC_input}
\end{figure}
\end{document}
